# Supplementary material for: Enriching Word Vectors with Subword Information
Source: arXiv:1607.04606 source file (2017-06-19)
Supplement: Supplementary file 1 [file appendix.tex]

\appendix

\section{Multi-threading}

We measure the performance of the obtained word vectors on the word similarity task, when the number of threads used for training change.
In Table~\ref{tab:threads} we report the correlation with human judgement for models trained on \texttt{small} for threads ranging from 1 to 32.
In Table~\ref{tab:threads-large} we report the correlation with human judgement for models trained on \texttt{large} for threads ranging from 15 to 30.

\begin{table}
  \centering
  \begin{tabular}{rcccccc}
    \toprule
    & 1 & 2 & 4 & 8 & 16 & 32 \\
    \midrule
de-gur350 & 68 & 67 & 69 & 67 & 68 & 69 \\
de-gur65 & 70 & 62 & 70 & 69 & 67 & 68 \\
de-zg222 & 49 & 41 & 43 & 44 & 45 & 48 \\
en-rw & 46 & 47 & 47 & 47 & 46 & 46 \\
en-ws353 & 62 & 63 & 63 & 64 & 63 & 64 \\
es-ws353 & 48 & 48 & 50 & 49 & 46 & 49 \\
fr-rg65 & 57 & 57 & 61 & 58 & 55 & 59 \\
    \bottomrule
  \end{tabular}
  \caption{
    Correlation between human judgement and our similarity for models trained on small with various number of threads.
  }
  \label{tab:threads}
\end{table}

\begin{table}
  \centering
  \begin{tabular}{rcccccc}
    \toprule
    & 15 & 20 & 25 & 30  \\
    \midrule
    de-gur350 & 68 & 68 & 67 & 68 \\
    de-gur65 & 72 & 77 & 74 & 75 \\
    de-zg222 & 41 & 40 & 44 & 43 \\
    en-rw & 46 & 46 & 46 & 46 \\
    en-ws353 & 65 & 66 & 67 & 66 \\
    es-ws353 & 53 & 53 & 51 & 53 \\
    fr-rg65 & 56 & 58 & 55 & 55 \\
    \bottomrule
  \end{tabular}
  \caption{
    Correlation between human judgement and our similarity for models trained on large with various number of threads.
  }
  \label{tab:threads-large}
\end{table}
